# Supplementary material for: Coupled dynamics of flow, microstructure, and conductivity in sheared suspensions
Source: arXiv:1602.05274 source file (2016-02-17)
Supplement: Supplementary file 1 [file supplemental_material.pdf]

# Coupled dynamics of flow, microstructure, and conductivity in sheared suspensions Supplementary Material

Tyler Olsen, Ahmed Helal, Gareth McKinley, and Ken Kamrin*
*Massachusetts Institute of Technology, Department of Mechanical Engineering*

## CONSTRAINT DERIVATIONS

This section lays out in more detail the derivation of constraints on the fabric tensor evolution law below.

$$\mathring{\mathbf{A}} = c_1\mathbf{1} + c_2\mathbf{A} + c_3\mathbf{D}. \tag{S1}$$

### Trace Condition

To find the physical conditions on the coefficients in the evolution law, we take the trace of (S1) and solve for the steady-state trace of the fabric, $\mathrm{tr}\mathbf{A}_{ss}$. The flow is assumed to be incompressible, so $\mathrm{tr}\mathbf{D} = 0$. We observe that electrical conductivity never entirely shuts off, regardless of the imposed strain rate $|\mathbf{D}|$. According to (2) in the main text, this implies that $\mathrm{tr}\mathbf{A} > 2$. This restriction yields a constraint between $c_1$ and $c_2$.

$$0 = 3\,c_1 + c_2\,\mathrm{tr}\mathbf{A}_{ss} \tag{S2}$$

$$\mathrm{tr}\mathbf{A}_{ss} = -\frac{3\,c_1}{c_2} > 2 \tag{S3}$$

### Positive Semidefinite Constraint

The fabric tensor is by definition a symmetric, positive semi-definite tensor. Thus, we must ensure that under no circumstances will the evolution law violate this condition. We can write the fabric tensor as

$$\mathbf{A} = \mathbf{Q}\mathbf{\Lambda}\mathbf{Q}^T \tag{S4}$$

Where $\mathbf{Q}$ is the eigenvector matrix and $\mathbf{\Lambda}$ is a diagonal matrix of eigenvalues. The time derivative of this quantity, then, is

$$\dot{\mathbf{A}} = \mathbf{Q}\dot{\mathbf{\Lambda}}\mathbf{Q}^T + \dot{\mathbf{Q}}\mathbf{\Lambda}\mathbf{Q}^T + \mathbf{Q}\mathbf{\Lambda}\dot{\mathbf{Q}}^T \tag{S5}$$

This can be rewritten as

$$\dot{\mathbf{A}} = \mathbf{Q}\dot{\mathbf{\Lambda}}\mathbf{Q}^T + \mathbf{\Lambda}\mathbf{\Omega} - \mathbf{\Omega}\mathbf{\Lambda} \tag{S6}$$

where $\Omega = \dot{\mathbf{Q}}\mathbf{Q}^T$, the spin of the eigenvectors, is a skew-symmetric matrix.

Suppose that during flow one of the eigenvalues approaches zero. The condition that $\mathbf{A}$ always be positive semi-definite requires that the rate of change of that eigenvalue be greater than or equal to zero. Without loss of generality, we choose $\mathbf{\Lambda}_{11} = \lambda_1$, to be zero. Suppose also that our global basis was chosen such that, at the moment when $\lambda_1 = 0$, the eigenvectors were aligned with the global basis, so $\mathbf{Q} = \mathbf{1}$. The evolution for the $\lambda_1$ eigenvalue is

$$\dot{\lambda}_1 = c_1 + c_3 D_{11} \geq 0 \tag{S7}$$

Now, due to our constraint from Eq (6) in the main text, we know that $c_3$ is a negative-valued function, so we rewrite it as

$$\dot{\lambda}_1 = c_1 - \hat{c}_3 D_{11} \geq 0 \tag{S8}$$

where $\hat{c}_3$ is a positive-valued function.

It can be shown that for incompressible flow, $|\mathbf{D}| \geq \sqrt{\frac{3}{2}}|D_{11}|$. Therefore it is sufficient to find a relationship between $c_1$ and $\hat{c}_3$ that satisfies

$$c_1 - \hat{c}_3\sqrt{\frac{2}{3}}|\mathbf{D}| \geq 0 \tag{S9}$$

Solving, and substituting $c_3$ back in, we obtain the final form of the constraint.

$$\frac{c_1}{c_3} \leq -\sqrt{\frac{2}{3}}|\mathbf{D}| \tag{S10}$$

## DATA-FITTING ALGORITHM

**Algorithm 1** Computation of $\mathbf{A}_{ss}$ for given simple-shear flow with strain-rate $\dot{\gamma}$

**Input:** Simple-shear strain-rate $\dot{\gamma}$.
**Output:** Steady-state fabric $\mathbf{A}_{ss}$
Construct $\mathbf{L} = \dot{\gamma}\,\hat{x} \otimes \hat{y}$.
Define $\mathbf{D} = \frac{1}{2}\left(\mathbf{L} + \mathbf{L}^T\right)$, $\mathbf{W} = \frac{1}{2}\left(\mathbf{L} - \mathbf{L}^T\right)$.
Solve nonlinear equation for $\mathrm{tr}\mathbf{A}_{ss}$.
Compute $c_1$ and $c_2$ from $\mathrm{tr}\mathbf{A}_{ss}$ and $|\mathbf{D}|$
Use algebraic solution of (S1) with $\dot{\mathbf{A}} = 0$ to find $\mathbf{A}_{ss}$.

To fit the model, we minimize the squared error between the model prediction and experimental values. The procedure for calculating this error is given in algorithm 2.

**Algorithm 2** Objective function for evolution law optimization routine

**Input:** $Z_0$, $Z_\infty$, $\tau$, $\beta$, $\alpha$, $n$, $k_1$
**Output:** Squared error $=$ *Score*
  $Score \leftarrow 0$
  **for all** $\dot{\Gamma}_i \in$ {Experimental shear rates} **do**
    Compute $I_{ss}(\dot{\Gamma}_i)$ using (13) from main text and algorithm 1.
    Compute error between model and experiment:
    $err \leftarrow \left(I_{ss}(\dot{\Gamma}_i) - I_{exp}(\dot{\Gamma}_i)\right)^2$.
    $Score \leftarrow Score + err$
  **end for**
  **return** *Score*

The following algorithm outlines the high-level procedure for fitting the evolution law to a set of experimental data. It relies heavily on the preceeding procedures laid out in algorithm 1 and algorithm 2.

**Algorithm 3** Experimental fitting procedure

**Input:** List of $\{\dot{\Gamma}, I_{exp}\}$ pairs from steady-state experiments
**Output:** Evolution law coefficients $\{Z_0, Z_\infty, \tau, \beta, \alpha, n, \}$
  Estimate $b_1$ from relaxation time of transient ramp tests.
  Choose $n$ to match discrete particle simulations
  Call `fminunc` with objective function given by algorithm 2.
  $\{Z_0, Z_\infty, \tau, \beta, \alpha, n, \} \leftarrow$ Output from `fminunc`.
  Verify that all constraints are satisfied
  Adjust $b_1$ estimate and repeat until $\dot{\gamma}_0 = 0$ transient is well-matched.

## EXPERIMENTAL METHODS

The system studied is a carbon black suspension prepared in the absence of any dispersant by mixing carbon black particles (Cabot Vulcan XC72R of specific gravity 1.8) in a light mineral oil (Sigma-Aldrich, specific gravity 0.838, viscosity 20 mPa·s) as described in reference [1] at a weight concentration of 8%w/w. The suspension is sonicated for one hour and mixed vigorously prior to each test to minimize the effects of sedimentation.

Simultaneous rheo-electric measurements were performed using a custom setup on an ARG2 torsional stress-controlled rheometer with a parallel plate geometry. This setup uses liquid metal (EGaIn) to create a low-friction continuous electrical connection to the rotating shaft [2]. DC potentiostatic tests with $\phi = 100mV$ were performed using a Solartron SI1287 potentiostat. The plates ($d = 40mm$, $R_a = 0.10\mu m$), acting as a two-electrode system, are coated with gold to reduce contact resistance. All rheo-electric tests were performed at gap $h = 0.75mm$ and $T = 26 \pm 0.3°C$.

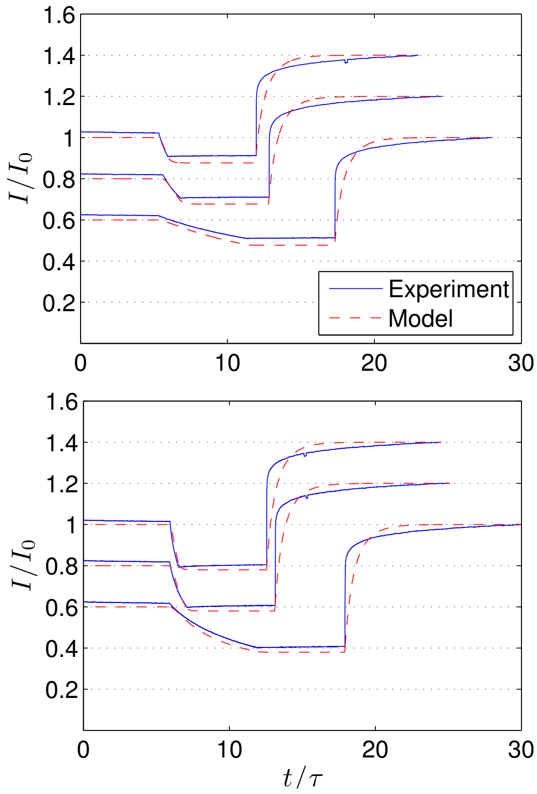


FIG. 1. Transient ramp experiments reproduced with the evolution law with $n = 0$. The model fails to adequately capture the relaxation behavior that occurs upon cessation of flow.

## LINEARIZED EVOLUTION LAW

In the main text, we assert that the evolution law with the power-law index $n$ set to 0 cannot capture the power-law relaxation behavior observed at low shear rates. The fabric relaxes at an exponential rate when $n = 0$, rather than at the power-law rate observed in our simulations. If we fit force $n = 0$ and refit the experimental data using teh fitting procedure, we obtain the parameters $Z_0 = 8.8$, $Z_\infty = 3.2$, $\tau = 1/50\,s^{-1}$, $\beta = 0.002$, $\alpha = -0.0026$, $n = 0$, and $k_1 = 0.0241\,S/m$.
The model is able to adequately reproduce the steady-state current measurements, but it fails to capture the relaxation upon cessation of flow. The results are shown in figure 1 of this supplement. Compare results to figure 4 in the main text.

* kkamrin@mit.edu

[1] V. Grenard, T. Divoux, N. Taberlet, and S. Manneville, Soft Matter **10**, 1555 (2014).
[2] A. Helal, T. Divoux, X. Chen, Y.-M. Chiang, and G. H. McKinley, Phys. Rev. Applied (InPreparation).
